# Supplementary material for: Context Aware Query Rewriting for Text Rankers using LLM
Source: arXiv:2308.16753 source file (2023-08-31)
Supplement: Supplementary file 1 [file appendix.tex]

\begin{supertabular}{llp{.70\textwidth}}
    \toprule 
    \textbf{Method}  & \textbf{Query id}    & \textbf{query text} \\
\midrule 
Original & 127392 & define sri \\
\vinci{} & 127392 & Sri is a Sanskrit word meaning “holy” or “auspicious.” It is often used in Hinduism as an honorific title for a deity or spiritual teacher. It is also used in Buddhist and Jain contexts, and is an important concept in South Asian culture. \\
\vinci{} (doc context) & 127392 & What is the meaning of Sanskrit word "Sri" and how is it used as a title of veneration? \\
ChatGPT & 127392 & Find the definition and meaning of the acronym SRI (Socially Responsible Investing). \\
\chatgpt{} (doc context) & 127392 & What is the meaning of the Sanskrit word "Sri" and how is it used in Indian subcontinent? \\
\midrule 
Original & 97047 & coniferous herbivore \\
\vinci{} & 97047 & Find information about coniferous herbivores \\
\vinci{} (doc context) & 97047 & What health concerns have been found in the coniferous forest that are of particular concern for spotted owls? \\
ChatGPT & 97047 & What types of animals feed on coniferous trees and how do they adapt to this diet? \\
\chatgpt{} (doc context) & 97047 & What kind of herbivores can be found in the coniferous forest? \\
\midrule 
Original & 57978 & cadaver tomb \\
\vinci{} & 57978 & Find information about cadaver tombs. \\
\vinci{} (doc context) & 57978 & What is a gisant and how does it relate to cadaver tombs? \\
ChatGPT & 57978 & What is a cadaver tomb and what is its historical significance? \\
\chatgpt{} (doc context) & 57978 & What is a cadaver tomb and what is its significance in the later Middle Ages? \\
\midrule 
Original & \textbf{181039} & ephesians 6:5-9 \\
\vinci{} & 181039 & Find information about Ephesians 6:5-9. \\
\vinci{} (doc context) & 181039 & 7 With good will render service, as to the Lord, and not to men, 8 knowing that whatever good thing each one does, this he will receive back from the Lord \\
ChatGPT & 181039 & What is the meaning and interpretation of Ephesians 6:5-9 in the Bible? \\
\chatgpt{} (doc context) & 181039 & How does the passage in Ephesians 6:5-9 instruct slaves to behave towards their masters? \\
\midrule 
Original & \textbf{480437} & price nrz \\
\vinci{} & 480437 & Find information on the Pricing of Non-Recourse Z-Bonds. \\
\vinci{} (doc context) & 480437 & What is the pricing of New Residential Investment Corp. common stock on Jan 30, 2017 7:16 PM EST? \\
ChatGPT & 480437 & Find information on the pricing strategy for non-return-to-zero (NRZ) encoding. \\
\chatgpt{} (doc context) & 480437 & What is the public offering price of New Residential Investment Corp.'s common stock? \\
\midrule 
Original & 1081897 & zeigarnik effect \\
\vinci{} & 1081897 & Find information about the Zeigarnik effect. \\
\vinci{} (doc context) & 1081897 & What are the implications of the Zeigarnik effect in Gestalt psychology? \\
ChatGPT & 1081897 & What is the Zeigarnik effect and how does it affect memory recall? \\
\chatgpt{} (doc context) & 1081897 & How does the Zeigarnik effect relate to memory retention and incomplete tasks? \\
\midrule 
Original & \textbf{525248} & tty number \\
\vinci{} & 525248 & Find information about how to locate a TTY number. \\
\vinci{} (doc context) & 525248 & What is the TTY number for Disability Services? \\
ChatGPT & 525248 & What is a TTY number and how is it used for communication? \\
\chatgpt{} (doc context) & 525248 & What are the TTY numbers for Ball State University's Switchboard and Disability Services office? \\
\midrule 
Original & 389096 & hs worms \\
\vinci{} & 389096 & Find information about heartworms in dogs. \\
\vinci{} (doc context) & 389096 & What are the courses offered by Hochschule Worms? \\
ChatGPT & 389096 & Find information about the symptoms, causes, and treatment of heartworm disease in dogs. \\
\chatgpt{} (doc context) & 389096 & What are the programs offered by Hochschule Worms? \\
\midrule 
Original & \textbf{89308} & ccm requirements\\
\vinci{} & 89308 & Find information about the requirements to become a Certified Case Manager (CCM).\\
\vinci{} (doc context) & 89308 & What educational qualifications and/or experience are required to become a Certified Construction Manager (CCM)?\\
ChatGPT & 89308 & What are the requirements for implementing a critical care management (CCM) program?\\
\chatgpt{} (doc context) & 89308 & What are the requirements to become a Certified Construction Manager (CCM)?\\
\midrule 
Original & 205430 & hornworms moth \\
\vinci{} & 205430 & Find information about the hornworms moth. \\
\vinci{} (doc context) & 205430 & What is the color and wing spread of the tomato hornworm moth? \\
ChatGPT & 205430 & What is the life cycle of hornworms moth and how do they affect crops? \\
\chatgpt{} (doc context) & 205430 & What is the appearance of an adult hornworm moth? \\
\midrule 
Original & 475948 & player is \\
\vinci{} & 475948 & Find information about the Player Is project. \\
\vinci{} (doc context) & 475948 & What types of players are involved in football, video games and other sports? \\
ChatGPT & 475948 & Find information about a player, including their stats, team history, and accomplishments. \\
\chatgpt{} (doc context) & 475948 & What are the different meanings of the term "player", including Football player, Gamer, Player character, Player-coach and Player \\
\midrule 
Original & 176525 & dunn effects \\
\vinci{} & 176525 & Find information on the effects of Dunn's law. \\
\vinci{} (doc context) & 176525 & What are the features of the Dunn O Effects Nyarlathotep distortion pedal? \\
ChatGPT & 176525 & Find information on the effects of Dunn's multiple comparison test in statistical analysis.\\
\chatgpt{} (doc context) & 176525 & What are the Dunn O Effects and how are they related to the Nyarlathotep distortion pedal? \\
\midrule 
Original & 186773 & figure pitch \\
DaVinci & 186773 & Find information about how to craft a successful pitch for a business figure. \\
\vinci{} (doc context) & 186773 & What is the method for figuring roof pitch? \\
ChatGPT & 186773 & Find information on what is meant by figure pitch and its significance in aircraft design. \\
\chatgpt{} (doc context) & 186773 & What is the method used by contractors and roof framers to figure a different pitch, or any roof pitch? \\
\midrule 
Original & 1168697 & urodeum function \\
DaVinci & 1168697 & Find information about the function of the urodeum in the digestive system \\
\vinci{} (doc context) & 1168697 & What is the purpose of accessory bladders or bursae in aquatic turtles? \\
ChatGPT & 1168697 & What is the function of the urodeum in avian anatomy? \\
\chatgpt{} (doc context) & 1168697 & What is the function of outpouchings from the lateral urodeal wall in aquatic turtles? \\
\midrule 
Original & 9631 & aam designation \\
DaVinci & 9631 & Find information about AAM (Advanced Accreditation Member) designation \\
\vinci{} (doc context) & 9631 & What is the process for obtaining the AAMS designation? \\
ChatGPT & 9631 & What does the AAM designation stand for and what are its requirements? \\
\chatgpt{} (doc context) & 9631 & What is the College for Financial Planning's Accredited Asset Management Specialist (AAMS) designation? \\
\midrule 
%\end{tabular}
%\caption{Comparing rewrites of ambiguous queries using \chatgpt{} and \vinci{} model with in-context and doc-context techniques.}
%\label{tab:rewriter_all_model_example_1}
\end{supertabular}
